# Supplementary material for: Lightweight Embeddings for Graph Collaborative Filtering
Source: arXiv:2403.18479 source file (2024-03-28)
Supplement: Supplementary file 1 [file appendices.tex]

\section{Appendix}

\subsection{Dimension Conversion for NGCF \& LR-GCCF} \label{sec:NGCF_LR_GCCF}
Since both NGCF and LR-GCCF generate the final GNN propagated embeddings by concatenating the embeddings obtained from each layer, the dimension size of the final GNN propagated embeddings will be different from the dimension size of the meta-codebook $\textbf{E}_{meta}$. In order to perform assignment update, we undertook empirical testing on pooling methods for the two base recommenders and decided to apply layer mean pooling to NGCF final embeddings and use the embeddings from the last layer of LR-GCCF to update the assignment matrix.
